# Supplementary material for: Adaptive Robust Model Predictive Control via Uncertainty Cancellation
Source: arXiv:2212.01371 source file (2022-12-02)
Supplement: Supplementary file 1 [file appendix.tex]

% \clearpage 
% \section{Appendix}



% \subsection{Empirical Estimator Comparison}
% We compare the set-membership and Bayesian least-squares estimators with each other. To do this, we generate samples of the nonlinear function
% \begin{align}
%     y^i  = w^\top \phi(x^i) + \epsilon^i = [w_1, w_2] \begin{bmatrix} \sin(4x_1) \\\frac{2}{\pi}\arctan(x_2^i)\end{bmatrix} + \epsilon^i
% \end{align}
% Here we take $\epsilon^i \sim U[-\sigma, \sigma]$. The initial feasible parameter sets are chosen as the unit box and unit circle respectively. We generate 30 samples and update the models iteratively. 
% \begin{figure}[t]
%     \centering
%     \includegraphics[width=.45\linewidth]{figures/estimators/set_membership_uniform.pdf}
%     \includegraphics[width=.45\linewidth]{figures/estimators/bayes_rls_uniform.pdf}
%     \caption{Recursive estimation of a nonlinear function.} 
%     \label{fig:est-nonlin}
% \end{figure}
% As shown in \cref{fig:est-nonlin}, with a well-specified model, the set-membership estimator outperforms RLS. However, the number of facets of the feasible parameter set can grow without bound, creating computational challenges. Moreover, since the confidence set can become arbitrarily small, the set membership estimator is not robust to outliers or model misspecification. We highlight this by adding a small bias $\alpha = .1$ to the mode. This is shown in figure \ref{fig:est-nonlin-biased}.
% \begin{figure}[t]
%     \centering
%         \includegraphics[width=.45\linewidth]{figures/estimators/set_membership_biased.pdf}
%         \includegraphics[width=.45\linewidth]{figures/estimators/bayes_rls_biased.pdf}
%     \caption{Recursive estimation of a nonlinear function with model misspecification.} 
%     \label{fig:est-nonlin-biased}
% \end{figure}
